# Supplementary material for: Decision-oriented two-parameter Fisher information sensitivity using symplectic decomposition
Source: arXiv:2207.12077 ancillary file (2022-10-12)
Supplement: Supplementary file 1 [file SymplecticFisherSensitivity_supplement.pdf]

# *Supplementary Material*: Decision-oriented two-parameter Fisher information sensitivity using symplectic decomposition

## 1 Computation of the symplectic eigenvectors

The symplectic eigenvectors cannot be solved using the standard eigenvalue algorithms directly. One approach uses the Schur form of skew-symmetric matrices and the symplectic eigenvector matrix can be found as:

$$\mathbf{S} = \mathbf{J}\mathbf{F}^{1/2}\mathbf{K}\mathbf{P}\begin{bmatrix} & -\mathbf{D}^{-1/2} \\ \mathbf{D}^{-1/2} & \end{bmatrix} \quad \text{(S1)}$$

The matrix $\mathbf{K}$ is a orthogonal matrix obtained from taking the Schur decomposition of the skew-symmetric matrix $\hat{\mathbf{F}} = \mathbf{F}^{1/2}\mathbf{J}\mathbf{F}^{1/2}$:

$$\mathbf{K}\hat{\mathbf{F}}\mathbf{K} = \mathrm{diag}\left(\begin{bmatrix} 0 & d_1 \\ -d_1 & 0 \end{bmatrix}, \ldots, \begin{bmatrix} 0 & d_n \\ -d_n & 0 \end{bmatrix}\right) \quad \text{(S2)}$$

and this can be done via the Matlab function ‘schur’ and the complex eigenvalues are put in 2-by-2 blocks on the diagonal as shown above (eigenvalues of a skew-symmetric matrix are pure imaginary). The matrix $\mathbf{P}$ is a permutation matrix to shuffle the eigenvalues:

$$\mathbf{P}^{\mathrm{T}}\mathbf{K}^{\mathrm{T}}\hat{\mathbf{F}}\mathbf{K}\mathbf{P} = \begin{bmatrix} & \mathbf{D} \\ -\mathbf{D} & \end{bmatrix} \quad \text{(S3)}$$

where

$$\mathbf{P} = [\mathbf{e}_1, \mathbf{e}_3, \ldots, \mathbf{e}_{2n-1}, \mathbf{e}_2, \mathbf{e}_4, \ldots, \mathbf{e}_{2n}] \quad \text{(S4)}$$

and $\mathbf{e}_j \in \mathbb{R}^{2n}$ is a unit vector with all zeros except the $j^{\text{th}}$ entry which is one.
It can be verified that the matrix given in Eq (S1) is symplectic and it diagonalize the matrix $\mathbf{F}$:

$$\begin{aligned} \mathbf{S}^{\mathrm{T}}\mathbf{F}\mathbf{S} &= \begin{bmatrix} & \mathbf{D}^{-1/2} \\ -\mathbf{D}^{-1/2} & \end{bmatrix}\mathbf{P}^{\mathrm{T}}\mathbf{K}^{\mathrm{T}}\mathbf{F}^{1/2}\mathbf{J}^{\mathrm{T}}\left(\mathbf{F}^{1/2}\mathbf{F}^{1/2}\right)\mathbf{J}\mathbf{F}^{1/2}\mathbf{K}\mathbf{P}\begin{bmatrix} & -\mathbf{D}^{-1/2} \\ \mathbf{D}^{-1/2} & \end{bmatrix} \\ &= \begin{bmatrix} & \mathbf{D}^{-1/2} \\ -\mathbf{D}^{-1/2} & \end{bmatrix}\left(-\mathbf{P}^{\mathrm{T}}\mathbf{K}^{\mathrm{T}}\hat{\mathbf{F}}\right)\left(\hat{\mathbf{F}}\mathbf{K}\mathbf{P}\right)\begin{bmatrix} & -\mathbf{D}^{-1/2} \\ \mathbf{D}^{-1/2} & \end{bmatrix} \\ &= \begin{bmatrix} & \mathbf{D}^{-1/2} \\ -\mathbf{D}^{-1/2} & \end{bmatrix}\begin{bmatrix} & -\mathbf{D} \\ \mathbf{D} & \end{bmatrix}(\mathbf{K}\mathbf{P})^{-1}(\mathbf{K}\mathbf{P})\begin{bmatrix} & \mathbf{D} \\ -\mathbf{D} & \end{bmatrix}\begin{bmatrix} & -\mathbf{D}^{-1/2} \\ \mathbf{D}^{-1/2} & \end{bmatrix} \\ &= \begin{bmatrix} \mathbf{D} & \\ & \mathbf{D} \end{bmatrix} \end{aligned} \quad \text{(S5)}$$

where the matrix $\mathbf{S}$ is substituted by the expression given in Eq (S1) at the first step. Then $\hat{\mathbf{F}} = \mathbf{F}^{1/2}\mathbf{J}\mathbf{F}^{1/2}$ is used at the second step, noting that $\mathbf{J}^{\mathrm{T}} = -\mathbf{J}$. At the third step, the expression in Eq (S3) is used with the fact that the matrix $\mathbf{K}\mathbf{P}$ is orthogonal. The above procedure is compiled in a Matlab function and the code is attached here for ease of reference.

```
function [S,D] = decomSymplect (F)
% input: SPD matrix
% output: S - Symplectic eigenvectors
%         D - Symplectic eigenvalues

% form the canonical symplectic matrix J
[N , ~] = size(F); % square matrix, N is even number
n = N/2;
J = [zeros(n) eye(n) ;...
    -eye(n)  zeros(n)];

% form skew-symmetric matrix Mt
M = F;
Ms = sqrtm(M); % sqrt of the matrix
Mt = Ms*J*Ms;
```

```
% Schur decomposition
[K,T] = schur(Mt);   % Q is orthogonal, T contains eigenvalues

% form permutation matrix
I = eye(N);
P = [I(:,1:2:2*n-1) I(:,2:2:2*n)];

% reshuffle the eigenvalue matrix
D2 = P.'*T*P;
D = abs(D2(1:n,n+1:2*n)); % diagonal

% form the symplectic matrix S
B = [zeros(n) -inv(sqrtm(D)) ; ...
    inv(sqrtm(D)) zeros(n)];
S = J*Ms*K*P*B;

% check that S is symplectic eigenvectors of F
% S'*J*S = J % symplecity
% S'*F*S = D % diagonal
```

## 2 Vibration of a thin cantilever beam

The mode shape for a thin cantilever beam is:

$$\begin{aligned}\phi_r(\xi) = \frac{C}{\sin\beta_r L - \sinh\beta_r L}\Big[&\left(\sin\beta_r L - \sinh\beta_r L\right)\left(\sin\beta_r\xi - \sinh\beta_r\xi\right) \\ &+\left(\cos\beta_r L + \cosh\beta_r L\right)\left(\cos\beta_r\xi - \cosh\beta_r\xi\right)\Big]\end{aligned} \tag{S6}$$

where $\beta_r, r = 1, 2, \ldots$ is the solution to the characteristic equation below:

$$\cos\beta L \cosh\beta L = -1 \tag{S7}$$

Solution of (S7) can be obtained numerically, e.g. Newton Raphson method, yielding an infinite set of $\beta_r$. It is assumed in the case study considered, only the first three modes are excited by the bandlimited white noise and the first three solutions are $\beta_1 L = 1.875$, $\beta_2 L = 4.694$ and $\beta_3 L = 7.855$.

The displacement frequency response function using modal summation is:

$$H_{\text{dis}}(\xi_{\text{re}}, \xi_{\text{ex}}, \omega) = \sum_{r=1} \frac{\phi_r(\xi_{\text{re}})\phi_r(\xi_{\text{ex}})}{\omega_r^2 - \omega^2 + 2i\zeta_r\omega_r\omega} \tag{S8}$$

where $\xi_{\text{re}}$ is the coordinate for the response measurement and $\xi_{\text{ex}}$ indicates the forcing position. $\zeta_r$ is the modal damping and it is assumed to be 0.1 for all modes and $\omega_r$ is the $r^{th}$ natural frequency given by:

$$\omega_r = (\beta_r L)^2 \sqrt{\frac{EI}{mL^4}} \tag{S9}$$

where $E$ is the Young's modulus, $I$ is the area moment of inertia and $m$ is the mass per unit length. Similarly, the frequency response function for strain is:

$$H_{\text{str}}(\xi_{\text{re}}, \xi_{\text{ex}}, \omega) = \sum_{r=1} \frac{\phi_r''(\xi_{\text{re}})\phi_r(\xi_{\text{ex}})}{\omega_r^2 - \omega^2 + 2i\zeta_r\omega_r\omega} \tag{S10}$$

Considering a white noise excitation $S_0$, the acceleration and strain response spectrum is given

$$S_{\text{acc}}(\xi_{\text{re}}, \xi_{\text{ex}}, \omega) = \left|\omega^2 H_{\text{dis}}\right|^2 S_0(\xi_{\text{ex}}) \tag{S11}$$

$$S_{\text{str}}(\xi_{\text{re}}, \xi_{\text{ex}}, \omega) = \left|H_{\text{str}}\right|^2 S_0(\xi_{\text{ex}}) \tag{S12}$$

The r.m.s response, for both acceleration and strain, can then be obtained as:

$$y(\xi) = \sqrt{\sum 2S(\xi, \omega)\,\mathrm{d}\omega} \tag{S13}$$

## 3 Results for the case study with proportionally normalised FIM

In this section, the numerical results is presented for the example considered in Section 4 of the *Main Text* for a proportionally normalised FIM ($\mathbf{F}_{\mathrm{nor},jk} = b_j b_k \mathbf{F}_{jk}$). Results from both the standard eigenvalue decomposition and the symplectic decomposition are presented below, in the same format as in Section 4. First thing to note is that the proportionally normalised FIM has fewer dominant eigenvalues, compared to the results in Section 4. For example, there are only one or two standard eigenvalues that are much larger than in the rest in Figure S 1, while for the standard deviation normalised results the first four eigenvalues dominates. It should be noted that the first four standard eigenvectors, and the first two pairs of symplectic eigenvectors, are presented below to be consistent with the results in Section 4, but the corresponding eigenvalue magnitudes are quite different in this case.

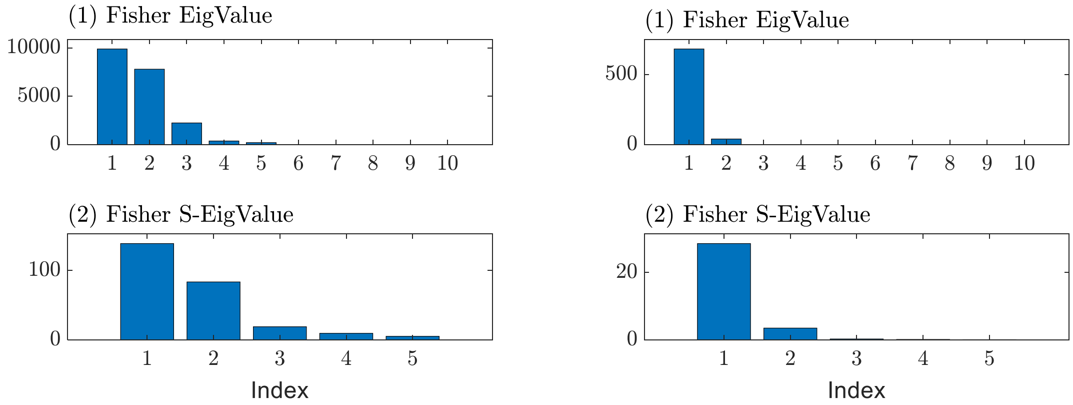


(a) Case-1 (b) Case-2

Figure S 1 Eigenvalues and symplectic eigenvalues of the proportionally normalised FIM

It can be seen from Figure S 2 and Figure S 3, as in Section 4, that the sensitivity information from the standard eigenvectors and the symplectic eigenvectors are similar, i.e., similar influential variables are identified. Except that the symplectic eigenvectors tend to group the parameters of the same variable. In addition, the standard eigenvectors tend to be dominated the mean values, in particular, all four eigenvectors for Case-1 point to the mean parameters as the influential ones. This can be understood as a consequence of the relatively large values of the mean parameters, as compared to the standard deviations (the standard deviations are typically a fraction of the mean values, c.f. Table 1 in the *Main Text*). As the proportional normalised FIM can be seen as sensitivity with respect to a percentage change of the parameters, the perturbation can be more significant for much larger values even the percentage change is the same. This might not be realistic practically, as unless the probability distribution of the input variables is far from the real distribution, it is most likely that the change of the mean should be within one or two standard deviation. As the symplectic decomposition is with respect to the two-parameter pairs, or the variable of interest, there is no need to distinguish the mean and the standard deviation. Therefore, for proportionally normalised FIM, the symplectic decomposition can also additional insights into the sensitivity analysis and should be used in tandem as the standard eigenvalue analysis.

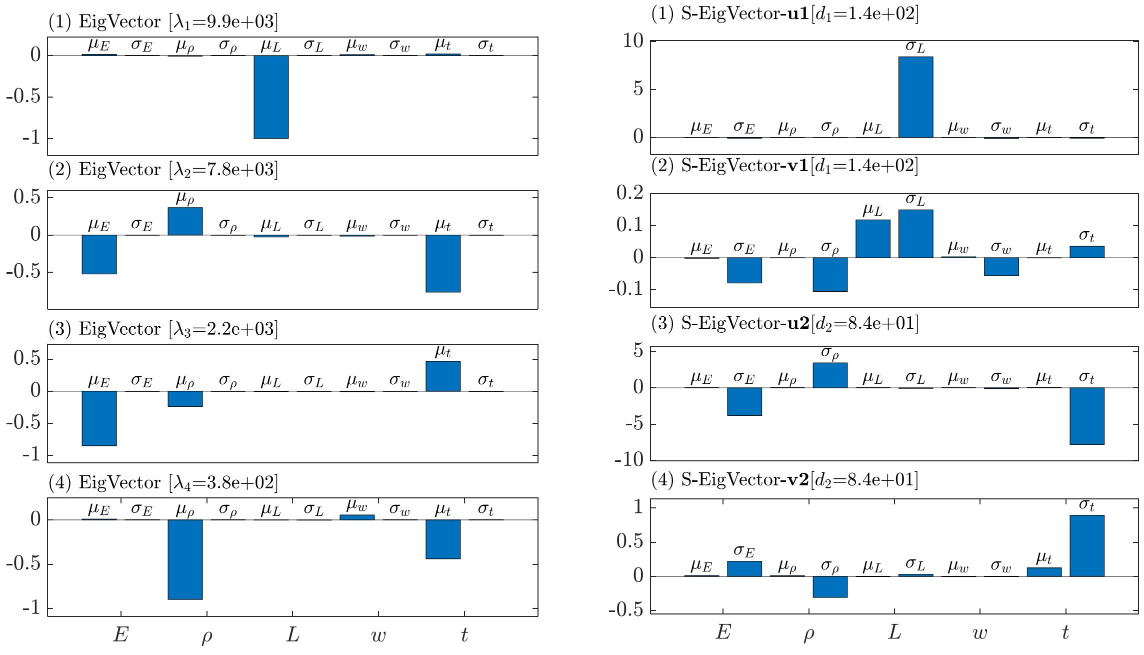


(a) standard eigenvectors (EigVector) (b) symplectic eigenvectors (S-EigVector)

Figure S 2 Eigenvectors (EigVector) and symplectic eigenvectors (S-EigVector) for *Case-1* listed in Table 1 in the *Main Text*, for a proportionally normalised FIM.

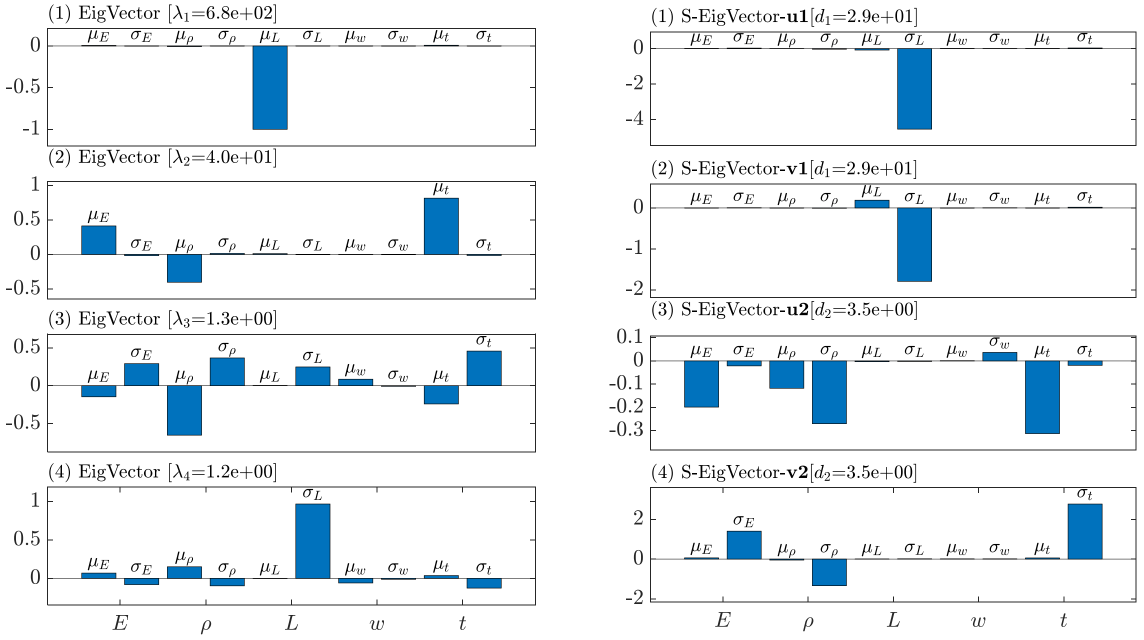


(a) standard eigenvectors (EigVector) (b) symplectic eigenvectors (S-EigVector)

Figure S 3 Eigenvectors (EigVector) and symplectic eigenvectors (S-EigVector) for *Case-2*, for a proportionally normalised FIM.
